# Supplementary material for: Analysis of Human Perception in Distinguishing Real and AI-Generated Faces: An Eye-Tracking Based Study
Source: arXiv:2409.15498 source file (2024-09-23)
Supplement: Supplementary file 1 [file supp_mat.tex]

\onecolumn
\setcounter{page}{1}
% \maketitlesupplementary
\section*{Supplementary Materials}
\setcounter{section}{0}

This supplementary document provides additional details on the data collection and data analysis and more, complementing the main text of our paper. The following sections offer deeper insights into our work.

\section{Instructions for Data Collection}

This section provides detailed instructions that all participant saw on the TV screen after calibration was done and before face images showed up. All participants saw 5 instruction pages as follows:

Page 1: ``Welcome to the experiment! Please press ENTER to continue."

Page 2: ``You will see one image of a human face on the screen. Your job is to look at the given image carefully, and decide whether it is an image of a real person (real image), or whether it is an image that is generated by a model (fake image)."

Page 3: ``Press 1 on the keyboard if you think it is a REAL image. Press 2 on the keyboard if you think it is a FAKE image."

Page 4: ``Press SPACE BAR to start!"

\section{Extra Details for Data Analysis}

% \subsection{Semantic Labels on 5 Attributes}

% Table~\ref{tab:attributes} shows the semantic meaning for each numerical label in each attribute.

% \begin{table}[H]
%     \centering
%     \begin{tabular}{|c|c|c|c|c|c|}
%     \hline
%     Attribute & 1 & 2 & 3 & 4 & 5  \\
%     \hline
%     Background & No & Yes & N/A & N/A & N/A \\
%     \hline
%     Gender & Male & Female & Uncertain & N/A & N/A \\
%     \hline
%     Skin Color & Light & Medium & Dark & Uncertain & N/A \\
%     \hline
%     Age & Child/Infant & Teen/Young Adult & Adult & Elderly & Uncertain \\
%     \hline
%     Accessory & Yes & No & Uncertain & N/A & N/A \\
%     \hline
         
%     \end{tabular}
%     \caption{Five attributes - numerical labels and their corresponding semantic labels. ``N/A" means a numerical label does not apply to this attribute; ``uncertain" means we could not assign a label for an attribute due to the quality of an image.} \label{tab:attributes}
% \end{table}

\subsection{Overall Spatial Density}

% \begin{figure}[h]
% \includegraphics[width=0.4
% \textwidth]{figs/all_density.jpg}
% \centering
% \caption{Average patch-wise fixation density on a grid of 4096 (64x64).}
% \label{patch_density}
% \end{figure}

% We also plot patch-wise fixation density by dividing an image into a grid of size 4096 (64 x 64). As shown in Figure~\ref{patch_density}, participants mostly looked at the center part of an image, which is where the face is located in most of the images.
